# Supplementary material for: Spams meet Cryptocurrencies: Sextortion in the Bitcoin Ecosystem
Source: arXiv:1908.01051 source file (2019-08-02)
Supplement: Supplementary file 1 [file appendix.tex]

% !TeX root = ../main.tex
% \section{Appendix}\label{sec:appendix}

% % \begin{longtable*}
% \input{sections/baskets_table}
% 	% \caption{Baskets} \\
% 	% \label{table:all_baskets} \\
% % \end{table*}
